# Supplementary material for: What Language Model Architecture and Pretraining Objective Work Best for Zero-Shot Generalization?
Source: arXiv:2204.05832 source file (2022-04-12)
Supplement: Supplementary file 1 [file scores.tex]

\begin{figure*}[h]
    \centering
    \includegraphics[width=\textwidth]{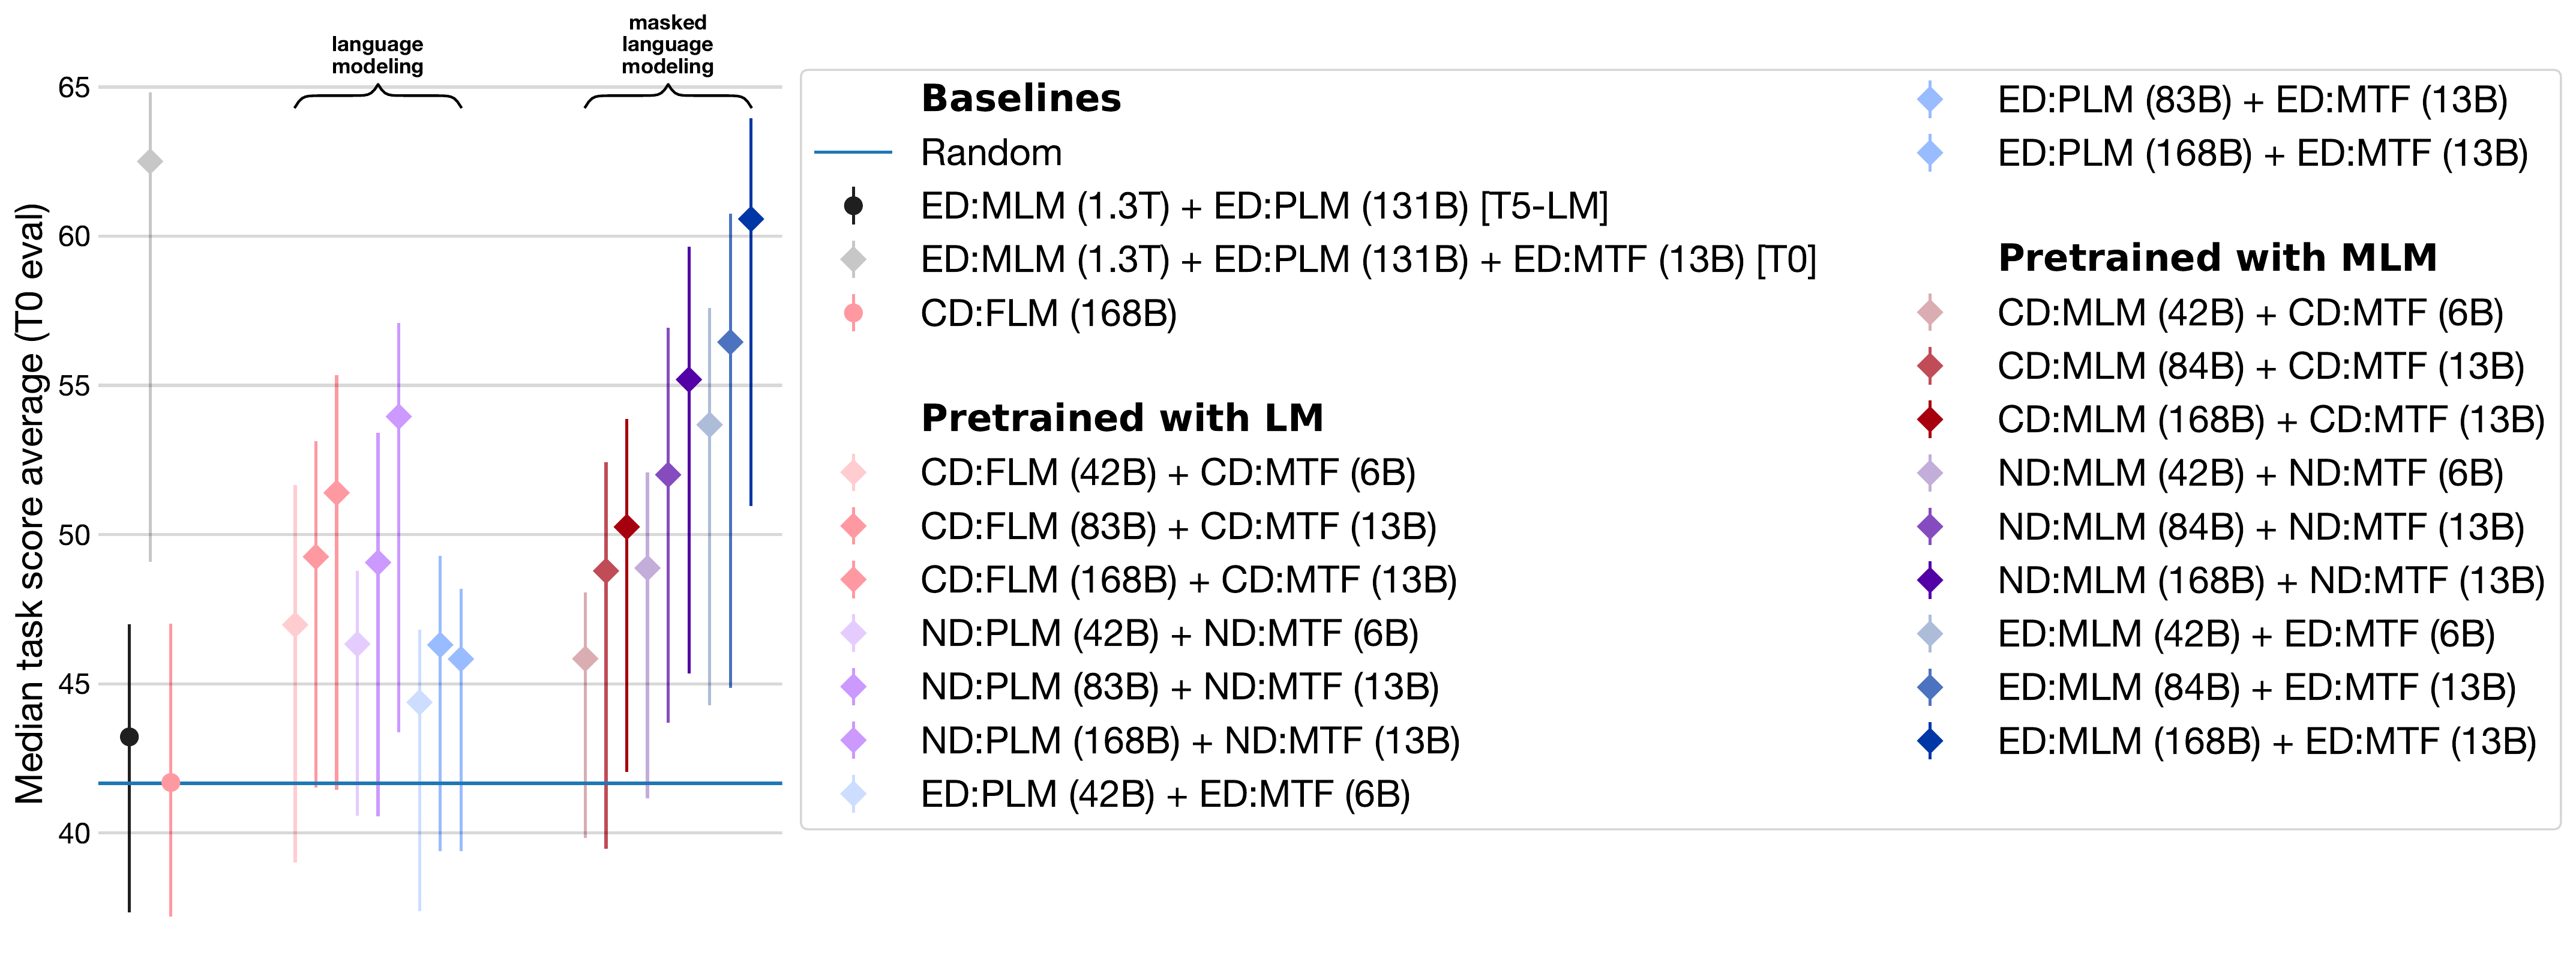}
    \caption{\textbf{Performance on the T0 evaluation set after T0 adaptation for increasing amounts of pre-training (measured in tokens), with unnormalized scores.} Difference with Figure \ref{fig:through_training} is minimal, and importantly does not impact ordering.}
    \label{fig:unnormalized}
\end{figure*}
